# Supplementary material for: Inferring COVID-19 Biological Pathways from Clinical Phenotypes via Topological Analysis
Source: arXiv:2101.07417 source file (2022-05-01)
Supplement: Supplementary file 1 [file doc-appendix.tex]

% %%
% %% If your work has an appendix, this is the place to put it.
% \appendix
% \section{Research Methods}
% \subsection{Part One}
% BLANK BLANK BLANK BLANK BLANK 
% \subsection{Part Two}
% BLANK BLANK BLANK BLANK BLANK 
% \section{Online Resources}
% BLANK BLANK BLANK BLANK BLANK 

{
	\small
	\begin{table}[H]
		\caption{Selected thirty-one ICD10-CM codes and the number of patients in each class} \label{Table:codes}
		\begin{center}
			\begin{tabular}{l@{\quad\quad}ll||l@{\quad\quad}ll}
				\hline
				\multicolumn{1}{l}{
					\textbf{ Description}}&\textbf{\scriptsize ICD10-CM}& \textbf{$\sharp$}&\textbf{\footnotesize Description}&\textbf{\scriptsize ICD10-CM}& \textbf{$\sharp$}\\[2pt]
				\hline
				Acute myocardial infarction & I21.9 &  5 & Chest pain & R07. &  24\\
				Pulmonary heart dis. & I27. &  6 & Abnormal sputum & R09.3 &  43\\
				Cardiac arrhythmia & I49.9 &  5& Nasal congestion & R09.81 &  11\\
				Heart failure& I50.9 &  9& Abdominal pain & R10.9 &  6\\
				Acute pharyngitis & J02.9 &  136& Nausea &R11. &  29\\
				Pneumonia & J18. &  151& Diarrhea &R19. &  28\\
				Nasal sinuses & J34.89 &  65& Dizziness &R42 &  6\\
				Respiratory failure & J96. &  64& Fever &R50.9 &  1073\\
				Pain in joint& M25.50 &  23& Headache &R51 &  76\\
				Muscle spasm & M62.838 &  24& Unspecified pain&R52 &  24\\
				Myalgia & M79.10 &  70& Fatigue &R53. &  177\\
				Disorders of bone & M89.8X9 &  10&Anorexia &R63.0 &  8\\
				Kidney failure & N17.9 &  9&Sepsis& R65.21 &  17\\
				Cough & R05 &  594& Chills &R68.83 &  41\\
				Abnormalities of breathing  & R06. &  138& Dry mouth &R68.2 &  6\\
				Sneezing & R06.7 &  17& &&\\		
				[2pt]\hline
			\end{tabular}
		\end{center}
	\end{table}
}
